# Supplementary material for: Bridging Queries and Tables through Entities in Table Retrieval
Source: arXiv:2504.06551 source file (2025-04-09)
Supplement: Supplementary file 1 [file appendix.tex]

% \onecolumn
\section{Instruction Details}
\label{app:instruction}
\subsection{Instruction of Listwise and Pointwise Approaches}
For the prompts of the NQ dataset using ChatGPT, we follow the setting of \citet{Zhang2024AreLL}, otherwise, we use the following prompts. 
Following \citet{sun2023chatgpt}, we input N passages using the form of multiple rounds of dialogue in the listwise approach. 
Considering the quality of the pseudo answer, we design a note, i.e., ``The reference answer may not be the correct answer, but it provides a pattern of the correct answer.'', adding before judging. 
We do experiments on listwise and pointwise respectively, and find that listwise is not sensitive to this note, note has a great influence on pointwise, as shown in Table \ref{tab:note_sep}
Finally, we choose prompt as shown in Figure \ref{fig:listwise-set-prompt} and Figure \ref{fig:pointwise-prompt}.
\begin{table}[htbp]
  \centering
    \begin{tabular}{ccccc}
    \toprule
      & \multicolumn{2}{c}{listwise}   & \multicolumn{2}{c}{pointwise} \\
    \cmidrule(r){2-3}   \cmidrule(r){4-5} 
    $m$     & $w.$ Note & $w/o$ Note & $w.$ Note& $w/o$ Note  \\
    \midrule
    $m$=1   & 53.56  & 53.91  & 49.44 & 48.34  \\
    $m$=2   & 55.30  & 55.65   & 51.09 & 49.44    \\
    $m$=3   & 54.57  & 54.86   & 51.74 & 50.02  \\
    $m$=4   & 53.87  & 55.02 & 51.90   & 50.30  \\
    $m$=5   & 53.99  & 54.86    & 51.65 & 50.60  \\
    \bottomrule
    \end{tabular}%
    \caption{Different F1 performance (\%) of \modelname using Mistral on TREC dataset in the listwise approach and the pointwise approach under different $m$ values between ``$w/o$ Note'', i.e.,  without the note and ''$w.$ Note'', i.e., with the note.}
  \label{tab:note_sep}%
\end{table}%

Moreover, for the implicit answer, we consider ``what information is necessary to answer the question'' and ``which information is necessary to answer the question'' in the prompt. Experiments are shown in Table \ref{tab:which_what}.
Finally, we choose prompt as shown in Figure \ref{fig:imp-answer-prompt}. 
For the experiments of ChatGPT API,  we have the cost of approximately \$248.
\begin{table}[htbp]
  \centering
    \begin{tabular}{ccccc}
    \toprule
      & \multicolumn{2}{c}{\trec}   & \multicolumn{2}{c}{\webap} \\
    \cmidrule(r){2-3}   \cmidrule(r){4-5} 
    $m$     & $w.$ which & $w.$ what & $w.$ which & $w.$ what \\
    \midrule
    $m$=1   & 49.39 & 48.34 & 26.06 &  25.81 \\
    $m$=2   & 50.72 &  50.13 &  28.67 & 25.38  \\
    $m$=3   & 52.05  & 50.94  &  28.36 & 25.04  \\
    $m$=4   &  51.71 & 51.54  & 25.46 & 26.87  \\
    $m$=5   &  51.54 &  50.66  &  27.35 & 26.69 \\
    \bottomrule
    \end{tabular}%
    \caption{Different F1 performance (\%) of \modelname using Mistral on \trec dataset and \webap dataset in the listwise approach under different $m$ values between ``$w.$ which'' and ``$w.$ what''.}
  \label{tab:which_what}%
\end{table}%

\label{sec:app:instruction}
\begin{figure*}[htbp]
    \centering
    \includegraphics[width=\linewidth]{images/app_prompts/listwise-set-prompt.pdf}
    \vspace{-3mm}
    \caption{Instruction in the listwise approach.}
\vspace{-1mm}
    \label{fig:listwise-set-prompt}
\end{figure*}

\begin{figure*}[htbp]
    \centering
    \includegraphics[width=\linewidth]{images/app_prompts/pointwise-prompt.pdf}
    % \vspace{-3mm}
    \caption{Instruction in the pointwise approach.}
\vspace{-1mm}
    \label{fig:pointwise-prompt}
\end{figure*}

\begin{figure*}[htbp]
    \centering
    \includegraphics[width=\linewidth]{images/app_prompts/ranking_prompts.pdf}
    % \vspace{-3mm}
    \caption{Instruction of the relevance ranking approach in our \modelname.}
    % \vspace{-1mm}
    \label{fig:relevance-ranking}
\end{figure*}
\subsection{Instruction of the Ranking Approach}
\label{app:sec:ranking}
For RankGPT, we directly use the instruction of \citet{sun2023chatgpt} for relevance ranking, as shown in Figure \ref{fig:sun-rank-prompt}. 
For the relevance ranking in our \modelname, the instructions are shown in Figure \ref{fig:relevance-ranking} and Figure \ref{fig:utility-ranking}.

\begin{figure*}[h]
    \centering
    \small
    \includegraphics[width=\linewidth]{images/app_prompts/utility-ranking.pdf}
    % \vspace{-3mm}
    \caption{Instruction of the utility ranking approach in our \modelname.}
% \vspace{-1mm}
    \label{fig:utility-ranking}
\end{figure*}

\begin{figure*}[htbp]
    \centering
    \includegraphics[width=\linewidth]{images/app_prompts/sun_ranking.pdf}
    \vspace{-3mm}
    \caption{Instruction of the ranking approach in \citet{sun2023chatgpt}.}
\vspace{-1mm}
    \label{fig:sun-rank-prompt}
\end{figure*}

\subsection{Instruction of Answer Generation}
\citet{li2023llatrieval} utilize LLM to generate the missing information in the provided documents for the current question and then re-retrieve it as relevant feedback. 
Therefore, we have also designed two kinds of pseudo answers for utility judgments, i.e., 
\begin{enumerate*}[label=(\roman*)]
\item the explicit answer, which produces an answer based on the given information, and 
\item the implicit answer, which does not answer the question directly but gives the information necessary to answer the question.
\end{enumerate*}
For ``words/sentences'', the experiments found that the length of the explicit answers generated by Mistral using ``sentences'' is too long for factual questions, whereas Llama 3 and chatGPT use ``sentences`` to generate answers of moderate length.
So we only use ``words`` on the TREC dataset and the NQ dataset using Mistral. 
The two instructions are shown in Figure \ref{fig:exp-answer-prompt} and Figure \ref{fig:imp-answer-prompt}. 
\begin{figure*}[htbp]
    \centering
    \includegraphics[width=\linewidth]{images/app_prompts/answer_generation.pdf}
    \vspace{-3mm}
    \caption{Instruction of the explicit answer generation.}
\vspace{-1mm}
    \label{fig:exp-answer-prompt}
\end{figure*}

\begin{figure*}[htbp]
    \centering
    \includegraphics[width=\linewidth]{images/app_prompts/cot-answer-prompt.pdf}
    \vspace{-3mm}
    \caption{Instruction of the implicit answer generation.}
\vspace{-1mm}
    \label{fig:imp-answer-prompt}
\end{figure*}

\begin{table*}[htbp]
  \centering
  % \small
    
   \setlength\tabcolsep{2pt}
    \begin{tabular}{c ccc ccc ccc ccc}
    \toprule
    \multicolumn{1}{c}{\multirow{3}[6]{*}{Method}} & \multicolumn{6}{c}{TREC}                     & \multicolumn{6}{c}{WebAP} \\
\cmidrule(r){2-7}   \cmidrule(r){8-13}  \multicolumn{1}{c}{} & \multicolumn{3}{c}{listwise} & \multicolumn{3}{c}{pointwise} & \multicolumn{3}{c}{listwise} & \multicolumn{3}{c}{pointwise} \\
\cmidrule(r){2-4} \cmidrule(r){5-7} \cmidrule(r){8-10} \cmidrule(r){11-13}    \multicolumn{1}{c}{} & P     & R     & F1    & P     & R     & F1    & P     & R     & F1    & P     & R     & F1 \\
    \midrule
     Vanilla  & 36.82  & 60.13  & 45.67  & 29.92  & \textbf{91.61}  & 45.11  & 13.07  & 50.83  & 20.79  & 13.30  & 86.29  &  23.05 \\
    \midrule
     UJ-ExpA & 48.51  & 61.15  & 54.10  & 28.12  & 96.27  & 43.53  & 18.83  & 54.16  & 27.94  & 14.65  & \textbf{91.82}  & 25.27  \\
     UJ-ImpA  & 40.16  & 60.53  & 48.29  & 33.95  & 83.76  & 48.31  & 16.46  & 52.45  & 25.06  & 17.56  & 73.55  & 28.35  \\
     % 10-sampling  & 47.04  & 61.01  & 53.12  &       -    &  -     &    -       & 22.27  & 53.69  & 31.49  &     -    &  -     &    -    \\
      5-sampling  & 46.64 	 &59.56  &52.31  &     -    &  -     &    - 	 &	20.61 &56.22  &	30.16   &     -    &  -     &    -    \\
    \midrule
    \modelname-A$_s$ $w.$ ExpA ($m$=1) & 48.07  & 61.04  & 53.78  & 34.21  & 89.11  & 49.44  & 20.57  & 53.81  & 29.76  & 17.86  & 78.41  & 29.10  \\
    \modelname-A$_s$ $w.$ ExpA ($m$=2) & 50.58  & 61.86  & 55.65  & 35.87  & 88.73  & 51.09  & 21.11  & 50.85  & 29.83  & 18.27  & 82.00  & 29.88  \\
    \modelname-A$_s$ $w.$ ExpA ($m$=3) & 50.61  & 59.88  & 54.86  & 36.23  & 90.46  & 51.74  & 23.57  & 48.14  & 31.65  & 18.73  & 81.96  & 30.50  \\
    \modelname-A$_s$ $w.$ ExpA ($m$=4) & 50.01  & 61.15  & 55.02  & \textbf{36.41}  & 90.36  & \textbf{51.90}  & 21.44  & 44.62  & 28.96  & \textbf{19.19}  & 80.59  & \textbf{31.00}  \\
    \modelname-A$_s$ $w.$ ExpA ($m$=5) & 50.61  & 59.88  & 54.86  & 36.14  & 90.46  & 51.65  & 24.07  & 47.09  & 31.86  & 19.17  & 78.94  & 30.85  \\
    \midrule
    \modelname-A$_s$ $w.$ ImpA ($m$=1) & 39.97  & 64.62  & 49.39  & 30.98  & 89.38  & 46.01  & 16.88  & 57.13  & 26.06  & 17.10  & 81.65  & 28.28  \\
    \modelname-A$_s$ $w.$ ImpA ($m$=2) & 43.14  & 61.52  & 50.72  & 30.90  & 87.00  & 45.60  & 19.41  & 54.82  & 28.67  & 18.88  & 78.06  & 30.40  \\
    \modelname-A$_s$ $w.$ ImpA ($m$=3) & 44.43  & 62.82  & 52.05  & 31.68  & 87.99  & 46.59  & 19.21  & 54.20  & 28.36  & 18.69  & 77.77  & 30.13  \\
    \modelname-A$_s$ $w.$ ImpA ($m$=4) & 44.72  & 61.29  & 51.71  & 31.66  & 87.40  & 46.49  & 17.44  & 47.11  & 25.46  & 18.95  & 78.06  & 30.50  \\
    \modelname-A$_s$ $w.$ ImpA ($m$=5) & 44.63  & 60.98  & 51.54  & 31.80  & 89.32  & 46.91  & 18.98  & 48.88  & 27.35  & 19.05  & 76.69  & 30.52  \\
    \midrule
    \modelname-AR$_s$ ($m$=1) & 43.65  & 65.34  & 52.34  &     -    &  -     &    -     & 25.04  & \textbf{60.99}  & 35.50  &    -    &  -     &    -    \\
    \modelname-AR$_s$ ($m$=2) & 45.10  & 65.46  & 53.40  &      -    &  -     &    -     & 24.42  & 51.97  & 33.23  &     -    &  -     &    -    \\
    \modelname-AR$_s$  ($m$=3) & 49.07  & \textbf{65.96}  & 56.27  &      -    &  -     &    -    & \textbf{27.70}  & 55.95  & \textbf{37.06}  &  -    &  -     &    -    \\
    \modelname-AR$_s$  ($m$=4) & 50.96  & 62.32  & 56.07  &    -    &  -     &    -        & 23.77  & 53.40  & 32.90  &       -    &  -     &    -   \\
    \modelname-AR$_s$  ($m$=5) & \textbf{53.01}  & 63.60  & \textbf{57.82}  &     -    &  -     &    -     & 25.85  & 47.56  & 33.50  &     -    &  -     &    -   \\
    \bottomrule
    \end{tabular}%
    \caption{The utility judgments performance (\%) of Mistral on retrieval datasets (Numbers in parentheses represent $m$-values). Numbers in bold indicate the best performance.}
  \label{tab:app:msitral}%
\end{table*}%

% Table generated by Excel2LaTeX from sheet 'final(webap)'
\begin{table*}[htbp]
  \centering
  % \small
    
   \setlength\tabcolsep{2pt}
    \begin{tabular}{c ccc ccc ccc ccc}
    \toprule
       \multicolumn{1}{c}{\multirow{3}[6]{*}{Method}} & \multicolumn{6}{c}{TREC}                     & \multicolumn{6}{c}{WebAP} \\
\cmidrule(r){2-7}   \cmidrule(r){8-13}  \multicolumn{1}{c}{} & \multicolumn{3}{c}{listwise} & \multicolumn{3}{c}{pointwise} & \multicolumn{3}{c}{listwise} & \multicolumn{3}{c}{pointwise} \\
\cmidrule(r){2-4} \cmidrule(r){5-7} \cmidrule(r){8-10} \cmidrule(r){11-13}    \multicolumn{1}{c}{} & P     & R     & F1    & P     & R     & F1    & P     & R     & F1    & P     & R     & F1 \\
    \midrule
     Vanilla & 34.67  & \textbf{85.80}  & 49.39  & 31.42  & \textbf{98.47}  & 47.64  & 12.69  & 77.15  & 21.79  & 14.65  & \textbf{87.36}  & 25.09 \\
    \midrule
   UJ-ExpA & 39.21  & 80.98  & 52.83  & 38.27  & 90.15  & 53.73  & 16.32  & 77.92  & 26.99  & 18.04  & 77.15  & 29.25  \\
     UJ-ImpA  & 33.92  & 83.36  & 48.22  & 38.68  & 71.47  & 50.20  & 15.57  & \textbf{82.79}  & 26.22  & 17.22  & 47.61  & 25.29  \\
    % k-sampling  & 39.79  & 79.72  & 53.08  &       &       &       & 17.15  & 77.25  & 28.07  &       &       &  \\
   5-sampling  &  39.04  &	80.98  &	52.68 & - & - & -				& 17.52 	& 83.49 &	28.97 & - & - & - \\
    \midrule
    \modelname-A$_s$ $w.$ ExpA ($m$=1) & 39.68  & 82.88  & 53.66  & 37.58  & 84.84  & 52.09  & 17.54  & 63.67  & 27.50  & 19.65  & 74.31  & 31.08  \\
     \modelname-A$_s$ $w.$ ExpA ($m$=2)  & \textbf{42.35}  & 84.77  & \textbf{56.48}  & 38.25  & 84.58  & 52.68  & 17.39  & 60.25  & 26.99  & 20.23  & 73.01  & 31.68  \\
     \modelname-A$_s$ $w.$ ExpA ($m$=3)  & 42.00  & 84.15  & 56.03  & 37.84  & 85.50  & 52.46  & 19.12  & 62.87  & 29.32  & \textbf{20.91}  & 74.63  & 32.67  \\
     \modelname-A$_s$ $w.$ ExpA ($m$=4)  & 41.85  & 84.41  & 55.96  & 38.12  & 85.16  & 52.67  & 17.53  & 61.85  & 27.31  & 20.44  & 73.83  & 32.02  \\
     \modelname-A$_s$ $w.$ ExpA ($m$=5)  & 42.36  & 84.15  & 56.35  & 37.35  & 84.69  & 51.84  & 18.94  & 62.87  & 29.12  & 20.88  & 75.45  & \textbf{32.71}  \\
    \midrule
    \modelname-A$_s$ $w.$ ImpA ($m$=1) & 39.63  & 83.42  & 53.73  & 39.70  & 82.87  & 53.68  & 15.48  & 73.66  & 25.59  & 20.04  & 64.06  & 30.53  \\
    \modelname-A$_s$ $w.$ ImpA ($m$=2) & 38.75  & 85.63  & 53.35  & 38.15  & 82.36  & 52.14  & 15.50  & 76.47  & 25.77  & 18.54  & 62.69  & 28.62  \\
    \modelname-A$_s$ $w.$ ImpA ($m$=3) & 40.84  & 84.86  & 55.14  & 40.58  & 79.64  & 53.76  & 15.99  & 70.99  & 26.10  & 19.54  & 61.32  & 29.64  \\
    \modelname-A$_s$ $w.$ ImpA ($m$=4) & 38.88  & 82.74  & 52.90  & 39.34  & 81.74  & 53.12  & 15.03  & 74.41  & 25.01  & 19.72  & 59.95  & 29.68  \\
    \modelname-A$_s$ $w.$ ImpA ($m$=5) & 41.26  & 84.61  & 55.47  & \textbf{40.92}  & 82.14  & \textbf{54.63}  & 15.49  & 68.93  & 25.29  & 19.84  & 57.21  & 29.46  \\
    \midrule
    \modelname-AR$_s$ ($m$=1) & 34.53  & 84.17  & 48.97  &      -    &  -     &    -       & \textbf{20.05}  & 72.88  & \textbf{31.44}  &   -    &  -     &    -   \\
    \modelname-AR$_s$  ($m$=2)& 36.27  & 83.19  & 50.51   	    &   -    &  -     &    -       & 15.92  & 79.01  & 26.50  &       -    &  -     &    -   \\
    \modelname-AR$_s$   ($m$=3) & 38.04  & 82.68  & 52.10 &  -    &  -     &    -       & 17.93  & 76.87  & 29.08  &       -    &  -     &    -   \\
    \modelname-AR$_s$   ($m$=4) & 37.28  & 83.70  & 51.58    &   -    &  -     &    -      & 16.60  & 78.81  & 27.42  &      -    &  -     &    -   \\
    \modelname-AR$_s$   ($m$=5) & 40.25  & 81.37  & 53.86 &     -    &  -     &    -     & 17.04  & 74.83  & 27.75  &      -    &  -     &    -   \\
    \bottomrule
    \end{tabular}%
    \caption{The utility judgments performance (\%) of Llama 3 on retrieval datasets (Numbers in parentheses represent $m$-values). Numbers in bold indicate the best performance.}
  \label{tab:app:llaMa}%
\end{table*}%

\begin{table*}[htbp]
  \centering
  \small
    
   \setlength\tabcolsep{2pt}
    \begin{tabular}{cccc ccc ccc ccc}
    \toprule
        \multicolumn{1}{c}{\multirow{3}[6]{*}{Method}} & \multicolumn{6}{c}{TREC}                     & \multicolumn{6}{c}{WebAP} \\
\cmidrule(r){2-7}   \cmidrule(r){8-13}  \multicolumn{1}{c}{} & \multicolumn{3}{c}{listwise} & \multicolumn{3}{c}{pointwise} & \multicolumn{3}{c}{listwise} & \multicolumn{3}{c}{pointwise} \\
\cmidrule(r){2-4} \cmidrule(r){5-7} \cmidrule(r){8-10} \cmidrule(r){11-13}    \multicolumn{1}{c}{} & P     & R     & F1    & P     & R     & F1    & P     & R     & F1    & P     & R     & F1 \\
    \midrule
    Vanilla & 42.13  & \textbf{79.98}  & 55.19  & 33.86  & 94.40  & 49.84  & 17.13  & \textbf{83.45}  & 28.43  & 15.80  & \textbf{89.42}  & 26.85  \\
    \midrule
   UJ-ExpA & 45.74  & 77.36  & 57.49  & 32.06  & \textbf{96.19}  & 48.09  & 19.51  & 69.86  & 30.50  & 16.23  & 88.74  & 27.44  \\
    UJ-ImpA & 44.19  & 77.11  & 56.18  & 33.45  & 90.36  & 48.83  & 18.37  & 80.14  & 29.89  & 15.58  & 84.51  & 26.32  \\
    % 10-sampling & 52.56  & 76.29  & 62.24  &    -   &   -    &    -   & 21.99  & 70.24  & 33.49  &    -   &  -     &  -\\
   5-sampling & 50.78 &	74.77 &	60.49 	& - & - & - &			20.70 &	65.83 &	31.49 & - & - & - \\
    \midrule
    \modelname-A$_s$ $w.$ ExpA ($m$=1) & 55.55  & 71.48  & 62.52  & 37.83  & 91.94  & 53.61  & 26.74  & 59.45  & 36.89  & 19.73  & 84.95  & 32.02  \\
    \modelname-A$_s$ $w.$ ExpA ($m$=2) & 57.95  & 70.40  & 63.57  & 40.74  & 93.04  & 56.67  & 29.43  & 60.58  & 39.62  & 19.62  & 78.62  & 31.40  \\
    \modelname-A$_s$ $w.$ ExpA ($m$=3) & 58.36  & 68.88  & 63.18  & 40.00  & 91.88  & 55.74  & 29.30  & 60.91  & 39.57  & 19.80  & 76.20  & 31.43  \\
    \modelname-A$_s$ $w.$ ExpA ($m$=4) & \textbf{58.48}  & 70.67  & \textbf{64.00}  & 40.25  & 93.38  & 56.25  & 29.11  & 61.03  & 39.42  & 20.48  & 79.63  & 32.58  \\
    \modelname-A$_s$ $w.$ ExpA ($m$=5) & 58.34  & 69.69  & 63.51  & 39.29  & 92.16  & 55.09  & 29.76  & 60.68  & \textbf{39.93}  & 20.58  & 80.42  & \textbf{32.77}  \\
    \midrule
    \modelname-A$_s$ $w.$ ImpA ($m$=1) & 54.36  & 65.08  & 59.24  & 40.89  & 82.20  & 54.61  & 24.79  & 64.37  & 35.80  & 18.78  & 67.00  & 29.34  \\
    \modelname-A$_s$ $w.$ ImpA ($m$=2) & 55.88  & 63.11  & 59.27  & 43.32  & 83.13  & \textbf{56.96}  & 27.68  & 62.03  & 38.28  & 20.70  & 70.54  & 32.00  \\
    \modelname-A$_s$ $w.$ ImpA ($m$=3) & 57.33  & 64.17  & 60.56  & 41.66  & 80.48  & 54.90  & \textbf{30.01}  & 63.60  & 40.78  & 21.51  & 66.77  & 32.54  \\
   \modelname-A$_s$ $w.$ ImpA ($m$=4) & 55.98  & 62.24  & 58.95  & \textbf{42.34}  & 80.65  & 55.53  & 28.43  & 60.11  & 38.60  & 20.60  & 65.63  & 31.36  \\
    \modelname-A$_s$ $w.$ ImpA ($m$=5) & 56.63  & 62.19  & 59.28  & 41.49  & 83.57  & 55.45  & 29.05  & 60.66  & 39.29  & \textbf{21.51}  & 68.03  & 32.68  \\
    \midrule
    \modelname-AR$_s$ ($m$=1) & 51.94  & 76.90  & 62.00  &   -    &  -     &    -   & 25.32  & 65.84  & 36.58  &     -    &  -     &    -     \\
    \modelname-AR$_s$  ($m$=2) & 53.77  & 76.19  & 63.05  &   -    &  -     &    -    & 25.55  & 59.26  & 35.70  &   -    &  -     &    -     \\
    \modelname-AR$_s$   ($m$=3) & 52.41  & 74.04  & 61.37  &   -    &  -     &    -   & 27.61  & 63.96  & 38.58  &   -    &  -     &    -   \\
    \modelname-AR$_s$   ($m$=4) & 52.75  & 73.78  & 61.52  &     -    &  -     &    -      & 28.84  & 61.85  & 39.34  &     -    &  -     &    -   \\
    \modelname-AR$_s$   ($m$=5) & 52.77  & 76.28  & 62.39  &    -    &  -     &    -      & 28.76  & 62.54  & 39.40  &     -    &  -     &    -   \\
    \bottomrule
    \end{tabular}%
    \caption{The utility judgments performance of ChatGPT on retrieval datasets (Numbers in parentheses represent $m$-values). Numbers in bold indicate the best performance.}
  \label{tab:app:chatgpt}%
\end{table*}%

\subsection{Effect of Iteration Numbers}
\label{app:exp:m_values}
The performance of different LLMs in different datasets is shown in Table \ref{tab:app:msitral}, Table \ref{tab:app:llaMa}, Table \ref{tab:app:chatgpt}, and Table \ref{tab:app:nq}.
% and Table \ref{app:tab:iteration_rdif}.

\begin{table*}[htbp]
  \centering
    \begin{tabular}{ccccccc}
    \toprule
   \multirow{2}[3]{*}{References of RAG} & \multicolumn{2}{c}{Mistral} & \multicolumn{2}{c}{Llama 3} & \multicolumn{2}{c}{ChatGPT} \\
\cmidrule(r){2-3}   \cmidrule(r){4-5}  \cmidrule(r){6-7}       & EM    & F1    & EM    & F1 & EM    & F1\\
\midrule
    Golden Evidence & 46.09  & 62.59  & 64.45  & 76.64  & 66.40  & 76.86  \\
    RocketQAv2 & 31.58  & 47.69  & \textbf{50.96 } & 62.01  & 46.54  & 57.00  \\
    \midrule
    Vanilla & 31.16  & 47.43  & 49.09  & 60.56  & 48.52  & 58.64  \\
    UJ-ExpA & 32.76  & 48.46  & 49.63  & 61.10  & 47.72  & 58.01  \\
    UJ-ImpA & 30.67  & 46.83  & 48.88  & 60.26  & 49.01  & 59.30  \\
    5-sampling & 33.24  & 48.84  & 48.72  & 60.71  & 48.90  & 58.97  \\
    \midrule
    \modelname-A$_s$ $w.$ ExpA ($m$=1) & 32.98  & 49.00  & 50.16  & 61.88  & 49.38 & 59.78 \\
    \modelname-A$_s$ $w.$ ExpA ($m$=2) & \textbf{34.31} & \textbf{50.08} & 50.48  & \textbf{62.32} & 49.22  & 59.99  \\
    \modelname-A$_s$ $w.$ ExpA ($m$=3) & 33.73  & 49.63  & 50.27  & 62.09  & \textbf{49.69} & \textbf{60.18} \\
    \modelname-A$_s$ $w.$ ExpA ($m$=4) & 34.21  & 50.07  & 50.43  & 62.20  &    -   &  -\\
    \modelname-A$_s$ $w.$ ExpA ($m$=5) & 33.78  & 49.63  & 50.27  & 62.07  &  -     & - \\
    \midrule
    \modelname-A$_s$ $w.$ ImpA ($m$=1) & 32.17  & 48.51  & 50.37  & 61.89  & 48.75 & 58.99 \\
    \modelname-A$_s$ $w.$ ImpA ($m$=2) & 32.49  & 48.67 & 49.63  & 61.16  & 49.11 & 59.14 \\
    \modelname-A$_s$ $w.$ ImpA ($m$=3) & 32.39  & 48.47  & 49.68  & 61.48  & 48.69 & 58.94 \\
    \modelname-A$_s$ $w.$ ImpA ($m$=4) & 32.71  & 48.84  & 49.41  & 61.03  &   -   & - \\
    \modelname-A$_s$ $w.$ ImpA ($m$=5) & 32.33  & 48.44  & 49.73  & 61.42  &   -    & - \\
    \midrule
    \modelname-AR$_s$ ($m$=1) & 33.30  & 49.26  & 50.27  & 61.69  & 49.52 & 59.64 \\
    \modelname-AR$_s$ ($m$=2) & 33.57  & 49.16  & 50.70  & 61.92  & 49.01 & 59.75 \\
    \modelname-AR$_s$ ($m$=3) & 33.40  & 49.27  & 49.36  & 60.97  & 49.06 & 59.67 \\
    \modelname-AR$_s$ ($m$=4) & 33.46  & 49.24  & 49.84  & 61.54  &     -  & - \\
    \modelname-AR$_s$ ($m$=5) & 33.89  & 49.58  & 49.20  & 60.84  &     -  & - \\
    \bottomrule
    \end{tabular}%
   \caption{The answer generation performance (\%) of all LLMs in the listwise approach. Numbers in bold indicate the best performance except the answer performance using golden evidence. Due to the high cost of using ChatGPT, we only tested with $m$=1,2,3 on ChatGPT. }
  \label{tab:app:nq}%
\end{table*}%

\begin{table*}[htbp]
  \centering
  % \small
  %     \renewcommand{\arraystretch}{0.95}
  %  \setlength\tabcolsep{3.7pt}
    \begin{tabular}{c ccccc ccc}
    \toprule
    \multirow{2}[4]{*}{$k$, $m$} & \multicolumn{5}{c}{Ranking} & \multicolumn{3}{c}{Utility judgments} \\
\cmidrule(r){2-6}  \cmidrule(r){7-9}  & N@1  & N@3  & N@5  & N@10 & N@20 & P     & R     & F1 \\
    \midrule
    $k$=1, $m$=1 & 72.76  & 71.27  & 70.57  & 72.69  & 84.08  & 53.66  & 24.09  & 33.25  \\
    $k$=1, $m$=2 & 76.02  & 71.54  & 71.38  & 73.66  & 84.78  & 58.54  & 28.73  & 38.54  \\
    $k$=1, $m$=3 & 77.24  & 72.83  & 71.83  & 73.87  & 85.20  & \textbf{59.76} & 28.84  & 38.90  \\
    $k$=1, $m$=4 & 77.24  & 73.04  & 71.91  & 73.90  & 85.25  & 59.76  & 28.84  & 38.90  \\
    $k$=1, $m$=5 & 76.02  & 72.11  & 71.42  & 73.45  & 84.98  & 58.54  & 28.71  & 38.53  \\
    \midrule
    $k$=5, $m$=1 & 72.76  & 71.27  & 70.57  & 72.69  & 84.08  & 33.17  & 57.31  & 42.02  \\
    $k$=5, $m$=2 & 78.46  & 73.74  & 72.86  & 75.48  & 86.09  & 32.93  & 58.37  & 42.10  \\
    $k$=5, $m$=3 & 79.27  & 75.00  & 74.27  & 75.78  & 86.80  & 34.15  & 62.57  & 44.18  \\
    $k$=5, $m$=4 & 79.67  & 75.92  & \textbf{75.35} & \textbf{76.83} & \textbf{87.23} & 35.12  & 61.40  & \textbf{44.68} \\
   $k$=5, $m$=5 & 79.67  & 75.32  & 74.61  & 76.20  & 86.82  & 34.63  & 61.25  & 44.25  \\
    \midrule
    $k$=10, $m$=1 & 72.76  & 71.27  & 70.57  & 72.69  & 84.08  & 22.56  &  68.03 & 33.88  \\
    $k$=10, $m$=2 & 78.05  & 72.64  & 72.90  & 75.48  & 85.74  & 23.66  & 75.47  & 36.02  \\
   $k$=10, $m$=3 & \textbf{80.89} & \textbf{76.58} & 74.54  & 76.30  & 86.94  & 23.78  & \textbf{75.65}  & 36.19  \\
    $k$=10, $m$=4 & 78.05  & 74.70  & 72.85  & 75.12  & 85.72  & 24.51  & 74.17  & 36.85  \\
    $k$=10, $m$=5 & 79.67  & 75.60  & 74.84  & 76.54  & 86.88  & 23.66  & 74.42  & 35.90  \\
    \bottomrule
    \end{tabular}%
    \caption{The utility ranking performance and utility judgments performance of Mistral on \trec dataset in \modelname-A$_r$. ``N@k'' means ``NDCG@k''. Numbers in bold indicate the best performance.}
  \label{tab:app:p_values}%
\end{table*}%
\subsection{$k$ values in \modelname-A$_r$}
\label{app:p_values}
Different ranking performance of $k$ values in \modelname-A$_r$ is shown in Table \ref{tab:app:p_values}. 
Considering the performance of utility ranking and utility judgments, we set $k$=5.

\section{Case Study}
\label{app:case_study}
We show another case on the TREC dataset in Table \ref{fig:exp-case-1}.

\begin{figure*}[h]
    \centering
    \includegraphics[width=\linewidth]{images/case_study/good_case1.pdf}
    \vspace{-3mm}
    \caption{An example of our \modelname-A$_s$ using Mistral on the  TREC dataset.}
\vspace{-1mm}
    \label{fig:exp-case-1}
\end{figure*}

% \begin{figure*}[h]
%     \centering
%     \includegraphics[width=\linewidth]{images/case_study/good_case2.pdf}
%     \vspace{-3mm}
%     \caption{An example of our \modelname-A$_s$ using Mistral on the  TREC dataset.}
% \vspace{-1mm}
%     \label{fig:exp-case-2}
% \end{figure*}

\section{Annotations in NQ Dataset}
\label{app:annotation_nq}
To evaluate the performance of utility judgments under different values of $m$, we relabeled the retrieved passages following \citet{stelmakh2022asqa}. 
Specifically, we used a QA model based on RoBERTa \cite{liu2019roberta} to extract answers from the retrieved passages. 
A passage is considered utility if the extracted answers match the ground-truth answers. 
The advantage of this labeling method is its relatively high accuracy, while its disadvantage is the potentially low recall rate.
